# Supplementary material for: Text Generation: A Systematic Literature Review of Tasks, Evaluation, and Challenges
Source: arXiv:2405.15604 source file (2026-08-06)
Supplement: Supplementary file 1 [file 10_Appendix.tex]

\section{Influential Citations} \label{app:influential_citations}
These parameters are considered for the influential citations attribute from Semantic Scholar:
\begin{enumerate}
     \item Total amount of direct citations
     \item Direct citations per section
     \item Total amount of indirect citations (per  section)
     \item Author overlap
     \item Helpfulness
     \item Citation appears in table or caption
     \item Inverse of the length of the citing paper’s reference list
     \item Number of paper citations divided by all citations
     \item Abstract similarity
     \item PageRank score
     \item Total amount of citing papers after transitive closure
     \item Research subfield
\end{enumerate}
